# Supplementary material for: Gaussian states of continuous-variable quantum systems provide universal and versatile reservoir computing
Source: arXiv:2006.04821 ancillary file (2021-03-31)
Supplement: Supplementary file 1 [file SuppMat.pdf]

# Supplementary Information for Gaussian states of continuous-variable quantum systems provide universal and versatile reservoir computing

Johannes Nokkala,[1,*] Rodrigo Martínez-Peña,[1] Gian Luca Giorgi,[1]
Valentina Parigi,[2] Miguel C. Soriano,[1] and Roberta Zambrini[1]

[1]*Instituto de Física Interdisciplinar y Sistemas Complejos (IFISC, UIB-CSIC), Campus Universitat de les Illes Balears E-07122, Palma de Mallorca, Spain*
[2]*Laboratoire Kastler Brossel, Sorbonne Université, CNRS, ENS-PSL Research University, Collège de France; CC74 4 Place Jussieu, 75252 Paris, France*

## I. PRELIMINARY INGREDIENTS

The purpose of this Supplementary Material is to prove that the model of Eq.(4) in the main text forms a universal class for quantum reservoir computing. Universality in this context refers to the possibility of finding elements of our class that approximate a given time-invariant, causal and fading memory map with arbitrary precision, as defined in [1]. In the main text, we specify the two pieces we need to ensure it, namely Lemma 1 and the Universality Theorem. In the former, we obtain the conditions for Echo State Property (ESP) and Fading Memory Property (FMP), and in the latter we demonstrate that our class fulfills all the requirements of the Stone-Weierstass Theorem, proving the universality. These requirements are to form a polynomial algebra, to contain constant functionals and to possess the point separation property. All these requirements will be properly defined and demonstrated in their respective Sections below.

In what follows, we will elaborate all the needed ingredients and once we are ready, we will tackle the proofs of Lemma 1 and the Universality Theorem of the main text.

### A. Input space

We will make use of infinite real sequences of inputs defined as $\mathbf{s} = \{\dots, \mathbf{s}_{-1}, \mathbf{s}_0, \mathbf{s}_1, \dots\}$, where $\mathbf{s}_k \in \mathbb{R}^n$, $n$ is the dimension of the input vector and $k \in \mathbb{Z}$. We can also define the left and right infinite sequences: $\mathbf{s} = \{\dots, \mathbf{s}_{-1}, \mathbf{s}_0\}$ where $\mathbf{s}_k \in \mathbb{R}^n$ and $k \in \mathbb{Z}_- = \{\dots, -1, 0\}$, and $\mathbf{s} = \{\mathbf{s}_0, \mathbf{s}_1, \dots\}$ where $\mathbf{s}_k \in \mathbb{R}^n$ and $k \in \mathbb{Z}_+ = \{0, 1, \dots\}$.

Now we introduce the definition of the input space, that we name $K_J$, and we always use during the proofs. The input sequences are chosen uniformly bounded. Let $J > 0$, then

$$K_J := \{\mathbf{s} = \{\dots, \mathbf{s}_{-1}, \mathbf{s}_0\} | \mathbf{s}_k \in \mathbb{R}^n \text{ and } ||\mathbf{s}_k|| \leq J \text{ for all } k \in \mathbb{Z}_-\}\,. \tag{S-1}$$

We note that our proof of universality is for infinite real sequences of inputs as we do not restrict ourselves to a compact time interval. Actually, the extension to infinite sequences provides a more general framework where we will introduce the useful concept of fading memory [1]. Fading memory, as was pointed out in [2], optimizes the total capacity of reservoir computer (RC) systems to perform different tasks.

### B. The dynamical system

Our goal is to demonstrate that a family of RC systems formed by quantum harmonic oscillator networks with Gaussian states is universal. Recall from the main text that $\mathbf{x}_k^R$ and $\mathbf{x}_k^A$ are the forms of the reservoir and ancilla operators at timestep $k$, respectively. The corresponding covariance matrices are denoted by $\sigma(\mathbf{x}_k^R)$ and $\sigma(\mathbf{x}_k^A)$, while the first moments vectors are denoted by $\langle \mathbf{x}_k^R \rangle$ and $\langle \mathbf{x}_k^A \rangle$.

Consider some network of $N$ oscillators. The relation between $\mathbf{x}_k^R$ and $\mathbf{x}_k^A$ is given by Eq. (4) of the main text, where matrices $\mathbf{A}$ and $\mathbf{B}$ are induced by the network Hamiltonian and time between inputs according to Eq. (3) of the main text. In terms of covariance matrices and first moments vectors, we get

$$\begin{cases} \sigma(\mathbf{x}_k^R) = \mathbf{A}\sigma(\mathbf{x}_{k-1}^R)\mathbf{A}^\top + \mathbf{B}\sigma(\mathbf{x}_k^A)\mathbf{B}^\top, \\ \langle \mathbf{x}_k^R \rangle = \mathbf{A}\,\langle \mathbf{x}_{k-1}^R \rangle + \mathbf{B}\,\langle \mathbf{x}_k^A \rangle\,, \end{cases} \tag{S-2}$$

* johannes@ifisc.uib-csic.es

where $\sigma(\mathbf{x}_k^R)$ and $\langle \mathbf{x}_k^R \rangle$ have dimensions $2(N-1)\times 2(N-1)$ and $2(N-1)$, respectively. At each timestep $k$ the ancilla is prepared into a displaced squeezed thermal state according to the input $\mathbf{s}_k$. The explicit forms of $\sigma(\mathbf{x}_k^A)$ and $\langle \mathbf{x}_k^A \rangle$ read

$$\begin{cases} \sigma(\mathbf{x}_k^A) = (n_k + \frac{1}{2}) \begin{pmatrix} [\cosh(2r_k) + \cos(\varphi_k)\sinh(2r_k)]\Omega^{-1} & \sin(\varphi_k)\sinh(2r_k) \\ \sin(\varphi_k)\sinh(2r_k) & [\cosh(2r_k) - \cos(\varphi_k)\sinh(2r_k)]\Omega \end{pmatrix}, \\ \langle \mathbf{x}_k^A \rangle = \begin{pmatrix} |\alpha|_k \cos\left(\arg(\alpha)_k\right)\sqrt{2\Omega^{-1}} \\ |\alpha|_k \sin\left(\arg(\alpha)_k\right)\sqrt{2\Omega} \end{pmatrix}, \end{cases} \tag{S-3}$$

where $\Omega > 0$ is the frequency of the ancilla oscillator, $n_k$ are the thermal excitations, $r_k$ and $\varphi_k$ are the magnitude and phase of squeezing, respectively, and $|\alpha|_k$ and $(\arg(\alpha))_k$ are the magnitude and phase of displacement, respectively. In general, each of the parameters of the chosen state may be taken to be some function of the input $\mathbf{s}_k$, with the restriction that $n_k$, $r_k$ and $|\alpha|_k$ are non-negative. In what follows we either assume that these functions are continuous or consider encoding to just one of the parameters with a linear function while keeping the rest constant (vanishing or not), like in the main text.

For the sake of simplicity, we are going to focus on the covariance matrix ($\sigma$) in the following Sections; generalization of obtained theoretical results to reservoir computing with first moments vector is straightforward. Therefore, the RC system under study in the rest of the Supplementary Material will be

$$\begin{cases} \sigma(\mathbf{x}_k^R) = \mathbf{A}\sigma(\mathbf{x}_{k-1}^R)\mathbf{A}^\top + \mathbf{B}\sigma(\mathbf{x}_k^A)\mathbf{B}^\top, \\ o_k = h(\sigma(\mathbf{x}_k^R)), \end{cases} \tag{S-4}$$

where, with a slight abuse of notation, $h$ is taken to be a (real) polynomial of the elements of $\sigma(\mathbf{x}_k^R)$. We remark that Eq. (S-4) is continuous in both $\sigma(\mathbf{x}_{k-1}^R)$ and input. From now on, we will use a shorthand notation for the covariance matrices of reservoir and ancilla, which will be $\sigma_k^R$ and $\sigma_k^A$ respectively.

### C. Assumptions

Along this supplement we will make some assumptions. They all are reminded at the moment we use them, but we collect all these conditions here for the sake of clarity. The main assumption is that the inputs are uniformly bounded, as it is expressed in Eq.(S-1). We point out the possibility to extend to the case of almost surely bounded inputs [3], where results are identical.

For the ESP, we will require $K_J$ to be compact. This space can be seen as a space composed of an infinite product of closed balls $\overline{B_n(\mathbf{0}, J)} \subset \mathbb{R}^n$, with center in $\mathbf{0}$ and radius $J$. These closed balls are compact, and by the Tychonoff Theorem (see Theorem 37.3 in [4]), $K_J$ is compact with the product topology. Furthermore, Corollary 2.8 in [5] shows that the metric space $(K_J, ||\cdot||_w)$ with respect to a weighted norm $||\cdot||_w$ (defined properly later) is a compact metric space. The latter compactness property will be needed for the Stone-Weierstrass Theorem, since we use a version where we speak about functions defined in compact metric spaces.

Another important assumption is the continuity of the ancilla parameters with respect to the input. This leads to some necessary bounds for the ancilla matrix, as will be seen in the following Sections II A and II B.

## II. LEMMA 1

### A. The Echo State Property

A reservoir has the echo state property (ESP) if and only if the recurrence relation that defines the reservoir state has a solution that is uniquely determined by the input history at the limit of infinitely many inputs, and not on the initial reservoir state. In other words, there must exist a function $\mathcal{E}$ that depends only on past inputs and determines the state of the reservoir; such functions are known as echo functions since the state of a reservoir with ESP can be thought of as an echo of the input. In our case, this is written as

$$\sigma_k^R = \mathcal{E}(\cdots, \mathbf{s}_{k-1}, \mathbf{s}_k). \tag{S-5}$$

This equation implies that the reservoir can constitute a temporal map, or filter, described in "Reservoir computing theory" Section in the main text. It is also indispensable for probing FMP, as will be seen.

Our strategy to demonstrate the ESP will be the following: we will propose a filter (or echo function). If it is a solution of Eq. (S-4) and it is uniquely determined by the input sequence, then the system has the ESP.

Consider now some reservoir defined by Eq. (S-4). Let $\{\mathbf{s}_{k-m}, \cdots, \mathbf{s}_k\}$ be some finite input sequence with $m \in \mathbb{N}$ and $\sigma^R_{k-m-1}$ be an initial covariance matrix, and let $\sigma^R_k$ be the state after $k$ timesteps when starting from $\sigma^R_{k-m-1}$. Applying Eq. (S-4), we get

$$\sigma^R_k = \mathbf{A}^{m+1}\sigma^R_{k-m-1}(\mathbf{A}^\top)^{m+1} + \sum_{j=0}^{m} \mathbf{A}^j\mathbf{B}\sigma^A_{k-j}\mathbf{B}^\top(\mathbf{A}^\top)^j. \tag{S-6}$$

The ESP is defined for infinite input sequences. Therefore, we extend Eq. (S-6) for an arbitrary left-infinite sequence $\mathbf{s} = \{\cdots, \mathbf{s}_{k-m}, \cdots, \mathbf{s}_k, \cdots, \mathbf{s}_0\}$ such that

$$\sigma^R_k = \lim_{m\to\infty} \mathbf{A}^{m+1}\sigma^R_{k-m-1}(\mathbf{A}^\top)^{m+1} + \lim_{m\to\infty}\sum_{j=0}^{m} \mathbf{A}^j\mathbf{B}\sigma^A_{k-j}\mathbf{B}^\top(\mathbf{A}^\top)^j. \tag{S-7}$$

To be able to write our filter, the system cannot depend on the initial condition since it must depend only on the input sequence. The dependence on the initial condition of Eq. (S-7) can be removed invoking Theorem 5.6.12 in [6], which states that $\lim_{m\to\infty}\mathbf{A}^m = 0$ if and only if $\rho(\mathbf{A}) < 1$, where $\rho(\mathbf{A})$ is the spectral radius of $\mathbf{A}$. Then, under the condition $\rho(\mathbf{A}) < 1$, Eq. (S-4) can be written as

$$M^{\mathbf{A},\mathbf{B}}(\mathbf{s})_k = \sigma^R_k = \sum_{j=0}^{\infty} \mathbf{A}^j\mathbf{B}\sigma^A_{k-j}\mathbf{B}^\top(\mathbf{A}^\top)^j, \tag{S-8}$$

where filters of reservoir states will be denoted by $M^{\mathbf{A},\mathbf{B}}$, and superscripts $\mathbf{A}$ and $\mathbf{B}$ account for the dependence on those matrices. To be sure that this proposal is well defined, we prove that the infinite sum of the previous equation is convergent. Let $n, m \in \mathbb{N}$ be such that $n < m$ and let $S_n := \sum_{j=0}^{n} \mathbf{A}^j\mathbf{B}\sigma^A_{k-j}\mathbf{B}^\top(\mathbf{A}^\top)^j$. We will use a property of square matrices given in Theorem 3.5 in [7] and in a slightly different way in Corollary 5.6.13 in [6]. Namely, given any square complex matrix $\mathbf{A}$, any $\varepsilon > 0$ and any sub-multiplicative matrix norm, there exists a finite $C \geq 1$ such that $||\mathbf{A}^k|| \leq C(\rho(\mathbf{A}) + \varepsilon)^k$. We choose $\varepsilon$ such that $0 < \varepsilon < 1 - \rho(\mathbf{A})$. Let $\gamma = \rho(\mathbf{A}) + \varepsilon$. Then:

$$||S_n - S_m||_2 \leq ||\mathbf{B}||_2^2 D \sum_{j=n+1}^{m} ||\mathbf{A}^j||_2^2 \leq ||\mathbf{B}||_2^2 DC^2 \sum_{j=n+1}^{\infty} (\gamma^2)^j = ||\mathbf{B}||_2^2 DC^2 \frac{\gamma^{2(n+1)}}{1-\gamma^2}, \tag{S-9}$$

where $||\cdot||_2$ is the Frobenius norm ($\sqrt{\mathrm{tr}(\sigma^\dagger\sigma)}$, where $\sigma$ is an arbitrary matrix and $\sigma^\dagger$ is its conjugate transpose), and the ancilla states fulfill $||\sigma^A_{k-j}||_2 \leq D$. Here, $D$ is a coefficient that appears because of the compactness of the input space and the continuity of the functions Eq.(S-3) contains. The condition $\gamma < 1$ implies that $||S_n - S_m||_2 \to 0$ as $n \to \infty$ and hence $\{S_n\}_{n\in\mathbb{N}}$ is a Cauchy sequence that converges.

Then, as the condition of $\rho(\mathbf{A}) < 1$ guarantees the disappearance of the first term in Eq. (S-7) and the convergence of the remaining term (S-8), this provides a sufficient and necessary condition for ESP.

As a final remark, the demonstration of the ESP for our system depends on the compactness of the input space through the coefficient $D$ In Eq. (S-9), and in fact, the space of states the reservoir explores due to the input, a space that we will call $K_L$, is compact since it is the image of a compact space under a continuous map (see, for instance, Theorem 26.5 in [4]).

### B. Fading Memory Property

The last part of the proof of Lemma 1 in the main text is about the FMP. Fading memory means that two input sequences that are close in the recent past produce outputs that are close in the present. This is a stronger condition than the usual continuity as we will show next. Indeed, the difference between outputs is required to vanish not only in the limit of identical inputs (as for continuity), but also for different inputs, as far as their difference is far in the past. In fact, a fading memory map is continuous but it does not imply that it is true in the other way around. Although FMP is introduced as a necessary condition for demonstrating universality with compact input spaces as it was done in [1], it is also true that it has become an important physical characteristic of RC systems [8].

To demonstrate FMP (and actually to work with the Stone-Weierstrass Theorem) we will need to find a functional that can describe the dynamical system of Eq. (S-4). Our functional will be defined as the map $F_h^{\mathbf{A},\mathbf{B}} : K_J \to \mathbb{R}$,

where superscript and subscript account for the dependence on the parameters and output function of our reservoir respectively. Functionals $F$ differ from filters $M$ as the former relate the inputs to the output at a given step while the latter map the input sequence in the full output sequence. We remind that in Eq.(S-8) we already found a filter that represents the dynamics of the reservoir. This filter can be extended to the whole RC system including the output function $h$, denoted by $M_h^{\mathbf{A},\mathbf{B}}(\mathbf{s})_k = h(M^{\mathbf{A},\mathbf{B}}(\mathbf{s})_k)$. Between causal and time-invariant filters and functionals there is a bijection. Causality means that our filter only produce outputs that depend on present and past inputs (it cannot access to information in the future) and time-invariance means that there is no explicit dependence on time in the system. Taking a look at Eq.(S-2), it is clear that both conditions are fulfilled for our equations. Having a well defined causal and time-invariant filter $M_h^{\mathbf{A},\mathbf{B}}$, the existence of a functional $F_h^{\mathbf{A},\mathbf{B}}$ is guaranteed. Indeed, for left-infinite sequences functional and filter are related as $F_h^{\mathbf{A},\mathbf{B}}(\mathbf{s}) = M_h^{\mathbf{A},\mathbf{B}}(\mathbf{s})_0$.

A more formal definition of the FMP is required and for this purpose we introduce a tool allowing us to express the continuity in terms of the recent past, the weighted norm. Let $w : \mathbb{N} \to (0, 1]$ be a null sequence, that is, a sequence that starts from $w_0 = 1$ and decreases until $w_\infty = 0$. We will call it weighting sequence. Then, it is defined the associated weighted norm $||\cdot||_w$ with respect to the weighting sequence $w$:

$$||\mathbf{s}||_w := \sup_{k\in\mathbb{Z}_-} \{||\mathbf{s}_k w_{-k}||\}, \tag{S-10}$$

where $||\cdot||$ is the Euclidean norm in $\mathbb{R}^n$. We will say that our RC system has the FMP if there exists a weighting sequence such that the functional $F_h^{\mathbf{A},\mathbf{B}} : (K_J, ||\cdot||_w) \to \mathbb{R}$ is continuous, where $(K_J, ||\cdot||_w)$ is the compact metric space associated to the weighted norm $||\cdot||_w$. This is expressed as usually: for each input sequence $\mathbf{u} \in K_J$ and any $\epsilon > 0$, there exists a $\delta(\epsilon) > 0$ such that for each $\mathbf{s} \in K_J$

$$||\mathbf{u} - \mathbf{s}||_w < \delta(\epsilon), \text{ then } \left|F_h^{\mathbf{A},\mathbf{B}}(\mathbf{u}) - F_h^{\mathbf{A},\mathbf{B}}(\mathbf{s})\right| < \epsilon. \tag{S-11}$$

In particular, we can define the $\lambda$-exponential FMP when the weighting sequence $w$ is $w_k = \lambda^k$ for some $\lambda \in (0, 1)$ and for all $k \in \mathbb{N}$. We will show that our family of RC systems are $\lambda_p$-exponential fading memory functionals, with $\lambda_p := \gamma^p$ for any $p \in (0, 1)$ and where $\gamma = \rho(\mathbf{A}) + \varepsilon$ was defined in the previous Subsection. This would correspond to the weighting sequence $w_k^p := \gamma^{pk}$, that will be a null sequence for spectral radius $\rho(\mathbf{A}) < 1$, the condition assumed in Lemma 1. Let $||\cdot||_{w^p}$ be the associated weighted norm in $K_J$ and let $\mathbf{s} \in K_J$ be an arbitrary element. The continuity of the readout map $h$ implies that for any $\epsilon > 0$, there exists an element $\delta(\epsilon) > 0$ such that for any $\tilde{\sigma}_k^R = \sum_{j=0}^{\infty} \mathbf{A}^j \mathbf{B} \sigma^A(\mathbf{u}_{k-j}) \mathbf{B}^\top (\mathbf{A}^\top)^j$ with $\mathbf{u} \in K_J$ that satisfies

$$\left|\left|\tilde{\sigma}_k^R - \sum_{j=0}^{\infty} \mathbf{A}^j \mathbf{B} \sigma^A(\mathbf{s}_{k-j}) \mathbf{B}^\top (\mathbf{A}^\top)^j\right|\right|_2 < \delta(\epsilon), \text{ then } \left|h(\tilde{\sigma}_k^R) - h\left(\sum_{j=0}^{\infty} \mathbf{A}^j \mathbf{B} \sigma^A(\mathbf{s}_{k-j}) \mathbf{B}^\top (\mathbf{A}^\top)^j\right)\right| < \epsilon. \tag{S-12}$$

So starting from the hypothesis

$$||\mathbf{u} - \mathbf{s}||_{w^p} < \delta'(\epsilon) = \frac{\delta(\epsilon)[1 - \gamma^{1-p}]}{||\mathbf{B}||_2^2 D_L C^2}, \tag{S-13}$$

we will show that

$$\left|F_h^{\mathbf{A},\mathbf{B}}(\mathbf{u}) - F_h^{\mathbf{A},\mathbf{B}}(\mathbf{s})\right| < \epsilon, \tag{S-14}$$

where $D_L$ and $C$ are constants.

The demonstration follows as a $\delta$-$\epsilon$ proof:

*Proof.*

$$\left|\left|\sum_{j=0}^{\infty} \mathbf{A}^j \mathbf{B} \left(\sigma^A(\mathbf{u}_{k-j}) - \sigma^A(\mathbf{s}_{k-j})\right) \mathbf{B}^\top (\mathbf{A}^\top)^j\right|\right|_2 \leq \sum_{j=0}^{\infty} ||\mathbf{A}^j||_2^2 ||\mathbf{B}||_2^2 ||\sigma^A(\mathbf{u}_{k-j}) - \sigma^A(\mathbf{s}_{k-j})||_2$$
$$\leq ||\mathbf{B}||_2^2 C^2 \sum_{j=0}^{\infty} \gamma^j ||\sigma^A(\mathbf{u}_{k-j}) - \sigma^A(\mathbf{s}_{k-j})||_2 \leq ||\mathbf{B}||_2^2 D_L C^2 \sum_{j=0}^{\infty} \gamma^j ||\mathbf{u}_{k-j} - \mathbf{s}_{k-j}||,$$

where $C$ was defined in the previous Subsection and we have introduced the Lipschitz constant $D_L$ by

$$||\sigma^A(\mathbf{u}_{k-j}) - \sigma^A(\mathbf{s}_{k-j})||_2 \leq D_L ||\mathbf{u}_{k-j} - \mathbf{s}_{k-j}||. \tag{S-15}$$

This inequality is justified as follows. A function $f:\mathbb{R}\rightarrow\mathbb{R}$ is Lipschitz continuous, i.e. $|f(x)-f(y)|\leq c|x-y|$ where $c$ is a constant, if its first derivative is bounded. For a continuous and differentiable function taking input values from a compact space, the first derivative is always bounded. We can see that in the covariance matrix of Eq.(S-3) all the matrix elements are continuous and differentiable functions respect to the input. The Frobenius norm takes the square root of the sum of these matrix elements to the power of two. This combination of functions is still continuous and differentiable. Problems could only arise from square root at the origin because it has infinite slope, but the function $||\sigma^A(\mathbf{s}_{k-j})||_2$ will never reach the origin since the zero matrix is not a valid covariance matrix.

Now we wish to introduce the weighted norm for the proof. For this purpose we need a closed form for the upper bound of the infinite sum. In [3] this step was carried out in Lemma 1:

$$||\mathbf{B}||_2^2 D_L C^2 \sum_{j=0}^{\infty}\gamma^j||\mathbf{u}_{k-j}-\mathbf{s}_{k-j}||\leq\frac{||\mathbf{B}||_2^2 D_L C^2||\mathbf{u}-\mathbf{s}||_{w^p}}{1-\gamma^{1-p}}<\delta(\epsilon).$$

This final step proves the continuity of the map $F_h^{\mathbf{A},\mathbf{B}}:(K_J,||\cdot||_{w^p})\rightarrow\mathbb{R}$ and hence $F_h^{\mathbf{A},\mathbf{B}}$ is a $\lambda_p$-exponential fading memory functional (Actually we proved the continuity of the associated filter, but this extends to functionals by virtue of the bijection mentioned before). The family of functionals $F_h^{\mathbf{A},\mathbf{B}}$ given by Eq. (S-4) will be named $\mathcal{Q}$.

The previous demonstration of the FMP was accomplished for the weighting sequence $w^p$. However, using subsets of uniformly bounded sequences as $K_J$ and $K_L$, we are allowed to say that if there exists FMP for a given $w$, then the filters (and respective functionals) have the FMP with respect to any other weighting sequence (Proposition 2.11 in [5]).

Recall that FMP implies that the initial state will be forgotten. As we saw in the previous Subsection this happens if and only if $\rho(\mathbf{A})<1$, making it a necessary condition for FMP. Here we have shown that it is also a sufficient condition, finishing the proof of Lemma 1 in the main text. □

### C. Spectral radius and the maximum singular value

We already stressed that $\rho(\mathbf{A})<1$ is a sufficient and necessary condition for ESP. This is unlike the common situation in the reservoir computing literature. The common approach to guarantee ESP is to find a sufficient condition, for example, with the contraction property (see e.g. [5]). However, this property leads to conditions where the induced norms play a role. Indeed, for a linear system of equations as reservoir, the sufficient condition for ESP would be $|||\mathbf{A}|||_2=\sigma_{\max}(\mathbf{A})<1$ [3], where $|||\cdot|||_2$ is the norm induced by the Frobenius norm and $\sigma_{\max}(\mathbf{A})$ is the maximum singular value of matrix $\mathbf{A}$. This sufficient condition can be also applied to our system, since knowing that $\rho(\mathbf{A})\leq|||\mathbf{A}|||$ for all induced norm, the condition $\sigma_{\max}(\mathbf{A})<1$ is sufficient to obtain $\rho(\mathbf{A})<1$. But not in the other way around. Therefore, our condition enlarges the amount of systems we can use as reservoirs since there are more instances of systems with $\rho(\mathbf{A})<1$ than $\sigma_{\max}(\mathbf{A})<1$. And of course, the sufficient and necessary condition $\rho(\mathbf{A})<1$ can be also proved in the linear reservoir system.

## III. UNIVERSALITY THEOREM

We start the proof of the Universality Theorem in the main text showing the version of the Stone-Weierstrass that we used along the work (taken from Theorem 7.3.1 in [9]):

**Stone-Weierstrass Theorem.** *Let $E$ be a compact metric space and $\mathcal{C}(E)$ be the set of real-valued continuous functions defined on E. If a subalgebra $A$ of $\mathcal{C}(E)$ contains the constant functions and separates points of $E$, then $A$ is dense in $\mathcal{C}(E)$.*

The leading player in this theorem is the compact metric space, denoted by $E$ and referred as $(K_J,||\cdot||_w)$ in our context, whose compactness was already clarified in Section I C. Then, the set of real-valued continuous functions $\mathcal{C}(E)$ will be denoted by $(C^0(K_J),||\cdot||_w)$, and contains all the $w$-fading memory functionals. Our task is to prove three different things: $(i)$ our family of systems $\mathcal{Q}$ is able to form a polynomial subalgebra of $(C^0(K_J),||\cdot||_w)$, $(ii)$ this subalgebra contains constant functionals and $(iii)$ it separates points of $(K_J,||\cdot||_w)$.

### Polynomial Algebra

We want to show that the family $\mathcal{Q}$ forms a polynomial algebra, that we will denote by $\mathcal{A}(\mathcal{Q})$, using a product defined in the space of functionals. It is a closure definition similar to the one of vector spaces, since it requires the

elements to remain in the same set under linear combination, but we further require the product of elements of the algebra to do so. We take two RC systems $\sigma_k^{R1}$ and $\sigma_k^{R2}$ with their respective matrices $\mathbf{A}_1$, $\mathbf{B}_1$, $\mathbf{A}_2$ and $\mathbf{B}_2$, and with their respective polynomial readouts $h_1$ and $h_2$. We can write the combinations of functionals as follows:

$$F_{h_1}^{\mathbf{A}_1,\mathbf{B}_1} \cdot F_{h_2}^{\mathbf{A}_2,\mathbf{B}_2} = F_{h_1 \cdot h_2}^{\mathbf{A}',\mathbf{B}'}, \quad F_{h_1}^{\mathbf{A}_1,\mathbf{B}_1} + \lambda F_{h_2}^{\mathbf{A}_2,\mathbf{B}_2} = F_{h_1 \oplus \lambda h_2}^{\mathbf{A}',\mathbf{B}'}, \tag{S-16}$$

with $\lambda \in \mathbb{R}$ and where $\mathbf{A}'$and $\mathbf{B}'$ will be specified below.

Since we are considering more than one independent network (with their respective ancillae) we introduce spatial multiplexing in a manner similar to the approach discussed in [10]. We define a Hamiltonian of the form

$$H = \sum_{i=1}^{P} H_i, \tag{S-17}$$

where $H_i$ is the Hamiltonian of each network and $P$ the total number of independent networks. If we have two independent networks (or a disconnected network with two components) with two ancillae (one ancilla per network), then the corresponding matrix $\mathbf{A}'$ is given by $\mathbf{A}' = \mathbf{A}_1 \oplus \mathbf{A}_2$ and matrix $\mathbf{B}'$ given by $\mathbf{B}' = \mathbf{B}_1 \oplus \mathbf{B}_2$, where the indices would correspond to the respective networks. This comes from the fact that matrices $\mathbf{A}_1 \oplus \mathbf{A}_2$ and $\mathbf{B}_1 \oplus \mathbf{B}_2$ are still the blocks of a symplectic matrix of a network of harmonic oscillators (with two disconnected components in this case).

Then, the covariance matrix

$$\sigma_k^{R'} = (\mathbf{A}_1 \oplus \mathbf{A}_2)(\sigma_{k-1}^{R1} \oplus \sigma_{k-1}^{R2})(\mathbf{A}_1 \oplus \mathbf{A}_2)^\top + (\mathbf{B}_1 \oplus \mathbf{B}_2)(\sigma_k^{A} \oplus \sigma_k^{A})(\mathbf{B}_1 \oplus \mathbf{B}_2)^\top \tag{S-18}$$

represents the dynamics of both networks at the same time.

It is straightforward to see that everything we have demonstrated until now is compatible with the extension to spatial multiplexing, since we were studying the particular case of a single network ($P = 1$). There is a final point that we must remark: the polynomial algebra generated by a set formed by fading memory reservoir functionals is made of fading memory reservoir functionals. Indeed, we only need to point out that

$$\rho(\mathbf{A}_1 \oplus \mathbf{A}_2) = \max\left(\rho(\mathbf{A}_1), \rho(\mathbf{A}_2)\right) < 1, \tag{S-19}$$

where we have taken $\rho(\mathbf{A}_1), \rho(\mathbf{A}_2) < 1$. The previous equation is true because the set of eigenvalues of $\mathbf{A}_1 \oplus \mathbf{A}_2$ is the union of the eigenvalues of $\mathbf{A}_1$ and $\mathbf{A}_2$.

### A. Constant functionals

Another demanded ingredient for the Stone-Weierstrass Theorem is to posses constant functionals in our polynomial algebra $\mathcal{A}(\mathcal{Q})$. As we are taking a polynomial readout, we can always take the polynomial of degree zero, i.e., a constant. So $\mathcal{A}(\mathcal{Q})$ contains constant functionals. This constant is usually known as the bias term in numerical simulations: it is essential to approximate functions with an offset with respect to the origin of their high dimensional spaces.

### B. Point Separation Property

The last part of the demonstration of Universality Theorem in the main text is to show that $\mathcal{A}(\mathcal{Q})$ separates points in $K_J$. It is enough to show that for any pair of points there is at least one element of the family that separates them. We can take the simplest situation: two oscillators, where one of them is the ancilla.

In the case of two harmonic oscillators with same natural frequency $\Omega > 0$ and coupling strength $g > 0$, the matrix $\mathbf{A}$ and $\mathbf{B}$ are the following:

$$\mathbf{A} = \frac{1}{2}\begin{pmatrix} \cos(\Omega_+\Delta t) + \cos(\Omega_-\Delta t) & \frac{1}{\Omega_+}\sin(\Omega_+\Delta t) + \frac{1}{\Omega_-}\sin(\Omega_-\Delta t) \\ -\Omega_+\sin(\Omega_+\Delta t) - \Omega_-\sin(\Omega_-\Delta t) & \cos(\Omega_+\Delta t) + \cos(\Omega_-\Delta t) \end{pmatrix} \equiv \begin{pmatrix} a_1 & a_2 \\ a_3 & a_1 \end{pmatrix}, \tag{S-20}$$

$$\mathbf{B} = \frac{1}{2}\begin{pmatrix} -\cos(\Omega_+\Delta t) + \cos(\Omega_-\Delta t) & -\frac{1}{\Omega_+}\sin(\Omega_+\Delta t) + \frac{1}{\Omega_-}\sin(\Omega_-\Delta t) \\ \Omega_+\sin(\Omega_+\Delta t) - \Omega_-\sin(\Omega_-\Delta t) & -\cos(\Omega_+\Delta t) + \cos(\Omega_-\Delta t) \end{pmatrix} \equiv \begin{pmatrix} b_1 & b_2 \\ b_3 & b_1 \end{pmatrix}, \tag{S-21}$$

where $\Omega_- = \Omega$ and $\Omega_+ = \sqrt{\Omega^2 + 2g}$ (with $\Omega_+ > \Omega_-$), and $\Delta t$ is the temporal interval between inputs. Take two input sequences $\mathbf{s}^1, \mathbf{s}^2 \in K_J$ such that $\mathbf{s}^1 \neq \mathbf{s}^2$. This means that there exists at least an index $i \in \{1, \ldots, n\}$ such that $s_k^{1i} \neq s_k^{2i}$ for some $k \in \mathbb{Z}_-$, where $s_k^i$ is the $i$-th component of the vector $\mathbf{s}_k$.

If we demonstrate that $M^{\mathbf{A},\mathbf{B}}(\mathbf{s}^1)_0 \neq M^{\mathbf{A},\mathbf{B}}(\mathbf{s}^2)_0$, we can take a linear readout and it follows that $M_h^{\mathbf{A},\mathbf{B}}(\mathbf{s}^1)_0 \neq M_h^{\mathbf{A},\mathbf{B}}(\mathbf{s}^2)_0$, or equivalently, $F_h^{\mathbf{A},\mathbf{B}}(\mathbf{s}^1) \neq F_h^{\mathbf{A},\mathbf{B}}(\mathbf{s}^2)$, as it was required for the point separation property.

Let us start computing $M^{\mathbf{A},\mathbf{B}}(\mathbf{s}^1)_0 - M^{\mathbf{A},\mathbf{B}}(\mathbf{s}^2)_0$:

$$M^{\mathbf{A},\mathbf{B}}(\mathbf{s}^1)_0 - M^{\mathbf{A},\mathbf{B}}(\mathbf{s}^2)_0 = \sum_{j=0}^{\infty} \mathbf{A}^j \mathbf{B}(\sigma^A(\mathbf{s}^1_{-j}) - \sigma^A(\mathbf{s}^2_{-j}))\mathbf{B}^\top(\mathbf{A}^\top)^j. \tag{S-22}$$

Since evaluating the previous infinite sum would be in general complicated, it is easier to find elements of the family that simplify the expression. The path we will follow consists of choosing the parameters $\Omega, \Delta t$ and $g$ in such a way that $\mathbf{A}$ is an anti-diagonal matrix which still fulfills $\rho(\mathbf{A}) < 1$. It might be expected that making $\mathbf{A}$ diagonal is a better choice but it would lead to $\rho(\mathbf{A}) = 1$. Choosing $g = \pi(\pi/2 + \Omega\Delta t)/(\Delta t)^2$, the matrices follow as

$$\mathbf{A} = \begin{pmatrix} 0 & \frac{\pi \sin(\Omega\Delta t)}{2\Delta t\Omega^2 + 2\pi\Omega} \\ \frac{\pi \sin(\Omega\Delta t)}{2\Delta t} & 0 \end{pmatrix}, \quad \mathbf{B} = \begin{pmatrix} \cos(\Omega\Delta t) & \frac{(2\Omega\Delta t+\pi)\sin(\Omega\Delta t)}{2\Omega(\Omega\Delta t+\pi)} \\ -\frac{(2\Omega\Delta t+\pi)\sin(\Omega\Delta t)}{2\Delta t} & \cos(\Omega\Delta t) \end{pmatrix}, \tag{S-23}$$

where we have total freedom over $\Omega$ and $\Delta t$, provided that they are positive.

The condition $\rho(\mathbf{A}) < 1$ has to be checked. In fact, since $\Omega, \Delta t > 0$ we have that $\rho(\mathbf{A}) = \sqrt{a_2 a_3}$ and consequently $\rho(\mathbf{A}) < 1$ whenever $a_2 a_3 < 1$. Given our choice of parameters,

$$a_2 a_3 = \frac{\pi^2 \sin^2(\Omega\Delta t)}{4\Omega\Delta t(\pi + \Omega\Delta t)}. \tag{S-24}$$

We remark that $0 \leq a_2 a_3 \leq \xi \approx 0.422$; importantly, it follows that $\rho(\mathbf{A}) < 1$ is ensured for any positive value of $\Omega$ and $\Delta t$.

Still we lack a final expression of the powers of $\mathbf{A}$. We can diagonalize it through

$$\mathbf{A} = \mathbf{K}\mathbf{\Lambda}\mathbf{K}^{-1}, \quad \mathbf{\Lambda} = \begin{pmatrix} -\sqrt{a_2 a_3} & 0 \\ 0 & \sqrt{a_2 a_3} \end{pmatrix}, \tag{S-25}$$

where $\mathbf{\Lambda}$ is the diagonal matrix and $\mathbf{K}$ the matrix of change of basis, which gives $\mathbf{A}^j = \mathbf{K}\mathbf{\Lambda}^j\mathbf{K}^{-1}$. Substituting in Eq.(S-22), we can rewrite it as

$$\begin{aligned} &M^{\mathbf{A},\mathbf{B}}(\mathbf{s}^1)_0 - M^{\mathbf{A},\mathbf{B}}(\mathbf{s}^2)_0 = \\ &\sum_{j=0}^{\infty} (a_2 a_3)^j \mathbf{K} \begin{pmatrix} (-1)^j & 0 \\ 0 & 1 \end{pmatrix} \mathbf{K}^{-1}\mathbf{B}(\sigma^A(\mathbf{s}^1_{-j}) - \sigma^A(\mathbf{s}^2_{-j}))\mathbf{B}^\top(\mathbf{K}^{-1})^\top \begin{pmatrix} (-1)^j & 0 \\ 0 & 1 \end{pmatrix} \mathbf{K}^\top. \end{aligned} \tag{S-26}$$

At this point, using the input as in Eq.(S-3), with all the parameters as a possible entry for the input, is a complicated way of tackling this problem. Below, we will specify which parameters and the type of encoding we use in order to evaluate Eq.(S-26).

1. **Thermal encoding**. Let us start with the simplest possible codification, that is the thermal input. We fix $r_k, \varphi_k = 0$. The input signal is introduced as $n_k = \mathbf{n}_{\text{th}} \cdot \mathbf{s}_k + n_{\text{th}0}$, where $\mathbf{n}_{\text{th}}$ and $n_{\text{th}0}$ are chosen such that $n_k > 0$. For convenience, we will take $\mathbf{n}_{\text{th}}$ as a zero vector, apart from a nonvanishing element in the entry $i$ (where inputs can be different). Using this encoding, we will demonstrate that the whole family $\mathcal{Q}$ can separate points, but at the same time we are also demonstrating that a much smaller family $\mathcal{Q}_{\text{thermal}}$ (the one given by thermal inputs) also separates points.

   For thermal encoding, matrix $\sigma^A_{-j}$ reduces to

$$\sigma^A_{-j} = (\mathbf{n}_{\text{th}} \cdot \mathbf{s}_{-j} + n_{\text{th}0} + \frac{1}{2}) \begin{pmatrix} 1/\Omega & 0 \\ 0 & \Omega \end{pmatrix}. \tag{S-27}$$

   Putting this expression in Eq. (S-26) we arrive at

$$\begin{aligned} M^{\mathbf{A},\mathbf{B}}(\mathbf{s}^1)_0 - M^{\mathbf{A},\mathbf{B}}(\mathbf{s}^2)_0 = &\sum_{j=0}^{\infty} (a_2 a_3)^j \mathbf{n}_{\text{th}} \cdot (\mathbf{s}^1_{-j} - \mathbf{s}^2_{-j}) \\ \times &\begin{pmatrix} \frac{-[-1+(-1)^j]a_2(b_3^2+b_1^2\Omega^2)+[1+(-1)^j]a_3(b_1^2+b_2^2\Omega^2)}{2a_3\Omega} & \frac{b_1(b_3+b_2\Omega^2)}{\Omega} \\ \frac{b_1(b_3+b_2\Omega^2)}{\Omega} & \frac{[1+(-1)^j]a_2(b_3^2+b_1^2\Omega^2)-[-1+(-1)^j]a_3(b_1^2+b_2^2\Omega^2)}{2a_2\Omega} \end{pmatrix}. \end{aligned} \tag{S-28}$$

We only need to show that just one of the matrix elements is nonvanishing in order to fulfill $M^{\mathbf{A},\mathbf{B}}(\mathbf{s}^1)_0 \neq M^{\mathbf{A},\mathbf{B}}(\mathbf{s}^2)_0$. So, we evaluate the off-diagonal term:

$$[M^{\mathbf{A},\mathbf{B}}(\mathbf{s}^1)_0 - M^{\mathbf{A},\mathbf{B}}(\mathbf{s}^2)_0]_{12} = -\frac{\pi(\pi + 2\Omega\Delta t)\sin(2\Omega\Delta t)}{4\Omega\Delta t(\pi + \Omega\Delta t)} \sum_{j=0}^{\infty} (a_2 a_3)^j \mathbf{n}_{\text{th}} \cdot (\mathbf{s}^1_{-j} - \mathbf{s}^2_{-j}), \tag{S-29}$$

where we have already substituted $b_1$, $b_2$ and $b_3$. At first sight, a necessary condition is to impose $2\Omega\Delta t \neq m\pi$, where $m$ is an integer, in order to to avoid $\sin(2\Omega\Delta t) = 0$. However, this condition is not sufficient, as in principle also the sum could be vanishing. We use a lemma from [11] (Theorem 3.2) for analyzing the infinite sum that will be the base of the demonstration.

**Lemma 2.** *Let $f_{\mathbf{c}}(x) := \sum_{j=0}^{\infty} c_{-j} x^j$ be a non-constant real power series, having a non-zero radius of convergence. If $f_{\mathbf{c}}(0) = 0$, then there exist a $\beta$ such that $f_{\mathbf{c}}(x) \neq 0$ for all $x$ with $|x| \leq \beta$ and $x \neq 0$.*

The fact that we need $f_{\mathbf{c}}(0) = 0$ in order to use this lemma makes us split the problem into two possible cases:

- $\mathbf{s}^1_0 = \mathbf{s}^2_0$. We can use Lemma 2, since $f_{\mathbf{c}}(0) = 0$. We have that $x = a_2 a_3 \in [0, \xi]$ and $|c_{-j}| = |\mathbf{n}_{\text{th}} \cdot (\mathbf{s}^1_{-j} - \mathbf{s}^2_{-j})| \leq 2Jn_{\text{th}}$, where $J$ is the bound introduced in $K_J$. Having $x < 1$ means that $f_{\mathbf{c}}(x)$ is always a convergent power series, and the radius of convergence for each $x$ must lay in the interval $(-2Jn_{\text{th}}, 2Jn_{\text{th}})$. So, invoking Lemma 2, we have that $f_{\mathbf{c}}(0) \neq 0$ for some $\beta$ such that $a_2 a_3 \leq \beta$. Now we have finished: an appropriate value of $a_2 a_3$ can always be achieved by tuning the parameters, since $a_2 a_3 \in [0, \xi]$ and is continuous in both $\Omega$ and $\Delta t$. Taking $h(\sigma^R_0) = [\sigma^R_0]_{12}$, we obtain $F^{\mathbf{A},\mathbf{B}}_h(\mathbf{s}^1) \neq F^{\mathbf{A},\mathbf{B}}_h(\mathbf{s}^2)$.
- $\mathbf{s}^1_0 \neq \mathbf{s}^2_0$. In this case, we cannot apply Lemma 2, since $f_{\mathbf{c}}(0) \neq 0$. However, we can follow an alternative strategy: if we put $\Delta t = \pi/\Omega$ in Eq. (S-23), which implies $g = 3\Omega^2/2$, we have $\mathbf{A} = 0$ and $\mathbf{B} = -\mathbf{I}$, where $\mathbf{I}$ is the identity matrix. Physically, this case corresponds to a swap Hamiltonian between the system oscillator and the ancilla. Implicitly, the filter of Eq. (S-8) is defined for $\mathbf{A} \neq 0$, but taking a look at Eq. (S-4) we can still define a filter for $\mathbf{A} = 0$ which trivially fulfill the conditions required until now. Then,

  $$M^{\mathbf{A},\mathbf{B}}(\mathbf{s}^1)_0 - M^{\mathbf{A},\mathbf{B}}(\mathbf{s}^2)_0 = n_{\text{th}}(s^{1i}_0 - s^{2i}_0) \begin{pmatrix} 1/\Omega & 0 \\ 0 & \Omega \end{pmatrix} \neq 0. \tag{S-30}$$

  It is straightforward to check that $F^{\mathbf{A},\mathbf{B}}_h(\mathbf{s}^1) \neq F^{\mathbf{A},\mathbf{B}}_h(\mathbf{s}^2)$ taking a linear readout with one of the diagonal elements of the reservoir state $h(\sigma^R_0) = [\sigma^R_0]_{ii}$.

2. **Squeezed encoding.** Once we have demonstrated separation of points for the family $\mathcal{Q}_{\text{thermal}}$ of thermal inputs, we want to do it for the family $\mathcal{Q}_{\text{squeezed}}$ of squeezed inputs as well. For squeezed encoding we fix $n_k, \varphi_k = 0$. The input signal is introduced as $r_k = \mathbf{r} \cdot \mathbf{s}_k + r_0$, where $\mathbf{r}$ and $r_0$ are chosen such that $r_k > 0$. For convenience, we choose $\mathbf{r}$ as a zero vector but with an element in the entry $i$. Matrix $\sigma^A_{-j}$ becomes

$$\sigma^A(\mathbf{s}_{-j}) = \frac{1}{2} \begin{pmatrix} e^{2(\mathbf{r}\cdot\mathbf{s}_{-j} + r_0)}/\Omega & 0 \\ 0 & \Omega e^{-2(\mathbf{r}\cdot\mathbf{s}_{-j} + r_0)} \end{pmatrix}, \tag{S-31}$$

and the difference between input matrices for two input sequences is

$$\sigma^A(\mathbf{s}^1_{-j}) - \sigma^A(\mathbf{s}^2_{-j}) = \sinh[\mathbf{r} \cdot (\mathbf{s}^1_{-j} - \mathbf{s}^2_{-j})] \begin{pmatrix} e^{\mathbf{r}\cdot\mathbf{s}^1_{-j} + \mathbf{r}\cdot\mathbf{s}^2_{-j} + 2r_0}/\Omega & 0 \\ 0 & -\Omega e^{-\mathbf{r}\cdot(\mathbf{s}^1_{-j} + \mathbf{s}^2_{-j})} \end{pmatrix}. \tag{S-32}$$

As in the thermal encoding case, we can calculate the matrix product of Eq.(S-26) and evaluate directly the off-diagonal term:

$$\begin{aligned} &[M^{\mathbf{A},\mathbf{B}}(\mathbf{s}^1)_0 - M^{\mathbf{A},\mathbf{B}}(\mathbf{s}^2)_0]_{12} = \\ &= -\sum_{j=0}^{\infty} (a_2 a_3)^j \sinh[r(s^{1i}_{-j} - s^{2i}_{-j})] \frac{\pi + 2\Omega\Delta t}{4\Omega\Delta t(\pi + \Omega\Delta t)} \\ &\times \left[\pi e^{\mathbf{r}\cdot\mathbf{s}^1_{-j} + \mathbf{r}\cdot\mathbf{s}^2_{-j} + 2r_0} + (e^{\mathbf{r}\cdot\mathbf{s}^1_{-j} + \mathbf{r}\cdot\mathbf{s}^2_{-j} + 2r_0} + e^{-\mathbf{r}\cdot(\mathbf{s}^1_{-j} + \mathbf{s}^2_{-j})})\Omega\Delta t\right] \sin(2\Omega\Delta t), \end{aligned} \tag{S-33}$$

where the new coefficients (i.e. all the factors apart from $x^j = (a_2a_3)^j$) fulfill $c_{-j} = 0$ when $\mathbf{s}^1_{-j} = \mathbf{s}^2_{-j}$ and $c_{-j} \neq 0$ when $\mathbf{s}^1_{-j} \neq \mathbf{s}^2_{-j}$ (since the large factor that comes along $\sinh[r(s^{1i}_{-j} - s^{2i}_{-j})]$ is always different from zero). Here we are considering again $2\Omega\Delta t \neq m\pi$ to avoid $\sin(2\Omega\Delta t) = 0$.

Now the demonstration is completely similar to the case of thermal encoding. If $\mathbf{s}^1_0 \neq \mathbf{s}^2_0$, we take $\mathbf{A} = 0$. If $\mathbf{s}^1_0 = \mathbf{s}^2_0$, we call again Lemma 2. We can apply it since we know that the coefficients $c_{-j}$ are bounded: they are continuous functions of the input, and the input is bounded.

3. **Phase encoding.** The separation of points is also possible for phase encoding. For the family $\mathcal{Q}_{\text{phase}}$ of phase inputs we fix $n_k = 0$ and we choose an arbitrary $r_k = r_0 > 0$. The input is given now by $\varphi_k = \mathbf{l} \cdot \mathbf{s}_k + \varphi_0$, and we choose $\mathbf{l}$ as a zero vector apart from a nonvanishing element in the entry $i$. Matrix $\sigma^A_{-j}$ becomes

$$\sigma^A(\mathbf{s}_{-j}) = \frac{1}{2}\begin{pmatrix} [p + q\cos(\mathbf{l}\cdot\mathbf{s}_{-j} + \varphi_0)]/\Omega & q\sin(\mathbf{l}\cdot\mathbf{s}_{-j} + \varphi_0) \\ q\sin(\mathbf{l}\cdot\mathbf{s}_{-j} + \varphi_0) & \Omega[p - q\cos(\mathbf{l}\cdot\mathbf{s}_{-j} + \varphi_0)] \end{pmatrix}, \tag{S-34}$$

where $p = \cosh(2r_0)$ and $q = \sinh(2r_0)$, and the difference between input matrices for two input sequences is

$$\begin{aligned} &\sigma^A(\mathbf{s}^1_{-j}) - \sigma^A(\mathbf{s}^2_{-j}) = \\ &q\sin[\frac{\mathbf{l}}{2}\cdot(\mathbf{s}^1_{-j} - \mathbf{s}^2_{-j})]\begin{pmatrix} -\frac{1}{\Omega}\sin[\frac{\mathbf{l}}{2}\cdot(\mathbf{s}^1_{-j} + \mathbf{s}^2_{-j}) + \varphi_0] & \cos[\frac{\mathbf{l}}{2}\cdot(\mathbf{s}^1_{-j} + \mathbf{s}^2_{-j}) + \varphi_0] \\ \cos[\frac{\mathbf{l}}{2}\cdot(\mathbf{s}^1_{-j} + \mathbf{s}^2_{-j}) + \varphi_0] & \Omega\sin[\frac{\mathbf{l}}{2}\cdot(\mathbf{s}^1_{-j} + \mathbf{s}^2_{-j}) + \varphi_0] \end{pmatrix}. \end{aligned} \tag{S-35}$$

Again, we can work out the solution Eq.(S-26) and evaluate the off-diagonal matrix element:

$$\begin{aligned} &[M^{\mathbf{A},\mathbf{B}}(\mathbf{s}^1)_0 - M^{\mathbf{A},\mathbf{B}}(\mathbf{s}^2)_0]_{12} = \\ &\sum_{j=0}^{\infty}(a_2a_3)^j q\sin[\frac{l}{2}(s^{1i}_{-j} - s^{2i}_{-j})] \\ &\times \frac{\left[\left(8\Omega^2\Delta t^2 + 8\pi\Omega\Delta t + \pi^2\right)\cos(2\Omega\Delta t) - \pi^2\right]\cos\left[\frac{l}{2}(s^{1i}_{-j} + s^{2i}_{-j}) + \varphi_0\right]}{8\Omega\Delta t(\Omega\Delta t + \pi)} \\ &+ \frac{2(2\Omega\Delta t + \pi)^2\sin(2\Omega\Delta t)\sin\left[\frac{l}{2}(s^{1i}_{-j} + s^{2i}_{-j}) + \varphi_0\right]}{8\Omega\Delta t(\Omega\Delta t + \pi)}, \end{aligned} \tag{S-36}$$

and the new coefficients fulfill $c_{-j} = 0$ when $\mathbf{s}^1_{-j} = \mathbf{s}^2_{-j}$ and $c_{-j} \neq 0$ when $\mathbf{s}^1_{-j} \neq \mathbf{s}^2_{-j}$, provided that some conditions are satisfied. It is clear that $c_{-j} = 0$ when $\mathbf{s}^1_{-j} = \mathbf{s}^2_{-j}$ because of the term $\sin[\frac{l}{2}(s^{1i}_{-j} - s^{2i}_{-j})]$. However, we need to choose the parameters $l$ and $\varphi_0$ in such a way that we get $c_{-j} \neq 0$ when $\mathbf{s}^1_{-j} \neq \mathbf{s}^2_{-j}$. This is always possible for any choice of the product $\Omega\Delta t$ since $\sin[\frac{l}{2}(s^{1i}_{-j} - s^{2i}_{-j})] = 0$ for $s^{1i}_{-j} \neq s^{2i}_{-j}$ can be avoided with $0 < l < \pi/J$, and then we can play with $l$ and $\varphi_0$ to avoid that the cosine and the sine factors of $c_{-j}$ vanish. Taking a smaller $l$, we shrink the window of possible values for $\frac{l}{2}(s^{1i}_{-j} + s^{2i}_{-j})$, and varying $\varphi_0$ we shift it.

Now the demonstration is completely similar to the other cases. If $\mathbf{s}^1_0 \neq \mathbf{s}^2_0$, we take $\mathbf{A} = 0$. If $\mathbf{s}^1_0 = \mathbf{s}^2_0$, we call Lemma 2. Again, the coefficients $c_{-j}$ are bounded because they are continuous functions of the input and the input is bounded.

Let us now state Universality Theorem of the main text in full:

**Universality Theorem.** *Given a uniformly bounded subset of input sequences $K_J$ and a null sequence $w$, fix $\Delta t$ and consider the family of functionals $F_h^{\boldsymbol{A},\boldsymbol{B}} : K_J \to \mathbb{R}$ called $\mathcal{Q}$ and associated with the instances of the reservoir system Eq.* (S-4) *for which $\rho(\boldsymbol{A}) < 1$, i.e. the functionals have the FMP with respect to a given weighted norm $||\cdot||_w$. Let $\mathcal{A}(\mathcal{Q})$ be their polynomial algebra. Then $\mathcal{A}(\mathcal{Q})$ has separability, and therefore any causal, time-invariant $w$-fading memory functional $F$ can be uniformly approximated by its elements. That is, for any causal, time-invariant $w$-fading memory functional, there exists $G \in \mathcal{A}(\mathcal{Q})$ such that for any $\varepsilon > 0$ and $\boldsymbol{s} \in K_J$, then*

$$||F - G||_\infty := \sup_{s\in K_J}\{|F(\boldsymbol{s}) - G(\boldsymbol{s})|\} < \varepsilon.$$

*In particular, this also holds for the subfamilies $\mathcal{Q}_{thermal}$, $\mathcal{Q}_{squeezed}$ and $\mathcal{Q}_{phase}$, that correspond to thermal, squeezed and phase encoding respectively.*

*Proof.* Applying Lemma 1 from the main text, we know that elements in $\mathcal{Q}$ have the FMP with respect to a given weighted norm $||\cdot||_w$. Then, as we have checked before, $\mathcal{A}(\mathcal{Q})$ is a subpolynomial algebra of the algebra $(C^0(K_J), ||\cdot||_w)$ of real valued continuous functions on $(K_J, ||\cdot||_w)$. We also proved that $\mathcal{A}(\mathcal{Q})$ contains the constant functionals and separate points in $K_J$. From Lemma 2 in [3], we know that the metric space $(K_J, ||\cdot||_w)$ is compact, so we can invoke the Stone-Weierstrass Theorem. This theorem implies that $\mathcal{A}(\mathcal{Q})$ is dense in $(C^0(K_J), ||\cdot||_w)$. In rough words, it means we can find elements that approximate with arbitrary precision functions from $(C^0(K_J), ||\cdot||_w)$, i.e., any causal and time-invariant $w$-fading memory map. In particular, this result is also true for the subfamilies $\mathcal{Q}_{\text{thermal}}, \mathcal{Q}_{\text{squeezing}}, \mathcal{Q}_{\text{phase}} \subset \mathcal{Q}$ of thermal, squeezing and phase encoding respectively. □

This Universality Theorem can be also applied for the first moments equation of the dynamical system in Eq.(S-2). The calculations do not differ much from the work above, and the possible encodings would be in the magnitude (encoding in $|\alpha|_k$ and $\arg(\alpha)_k = \text{const.}$) or the phase (encoding in $\arg(\alpha)_k$ and $|\alpha|_k = \text{const.}$) of displacement.

[1] S. Boyd and L. Chua, Fading memory and the problem of approximating nonlinear operators with volterra series, IEEE Transactions on circuits and systems **32**, 1150 (1985).
[2] J. Dambre, D. Verstraeten, B. Schrauwen, and S. Massar, Information processing capacity of dynamical systems, Scientific reports **2**, 514 (2012).
[3] L. Grigoryeva and J.-P. Ortega, Universal discrete-time reservoir computers with stochastic inputs and linear readouts using non-homogeneous state-affine systems, The Journal of Machine Learning Research **19**, 892 (2018).
[4] J. Munkres, *Topology* (Pearson Education, 2014).
[5] L. Grigoryeva and J.-P. Ortega, Echo state networks are universal, Neural Networks **108**, 495 (2018).
[6] R. A. Horn and C. R. Johnson, *Matrix analysis* (Cambridge university press, 2012).
[7] D. A. Dowler, *Bounding the norm of matrix powers*, Ph.D. thesis (2013).
[8] G. Tanaka, T. Yamane, J. B. Héroux, R. Nakane, N. Kanazawa, S. Takeda, H. Numata, D. Nakano, and A. Hirose, Recent advances in physical reservoir computing: A review, Neural Networks **115**, 100 (2019).
[9] J. Dieudonné, *Foundations of modern analysis* (Read Books Ltd, 2011).
[10] K. Nakajima, K. Fujii, M. Negoro, K. Mitarai, and M. Kitagawa, Boosting computational power through spatial multiplexing in quantum reservoir computing, Physical Review Applied **11**, 034021 (2019).
[11] S. Lang, *Complex analysis*, Vol. 103 (Springer Science & Business Media, 2013).
